# Supplementary material for: Collective behavior of bulk nanobubbles produced by the alternating polarity electrolysis
Source: arXiv:1712.08728 source file (2017-12-23)
Supplement: Supplementary file 1 [file Supplemental.pdf]

Electronic Supplementary Information

## Collective Behavior of Bulk Nanobubbles Produced by the Alternating Polarity Electrolysis

Alexander V. Postnikov, Ilia V. Uvarov, Nikita V. Penkov, Vitaly B. Svetovoy*

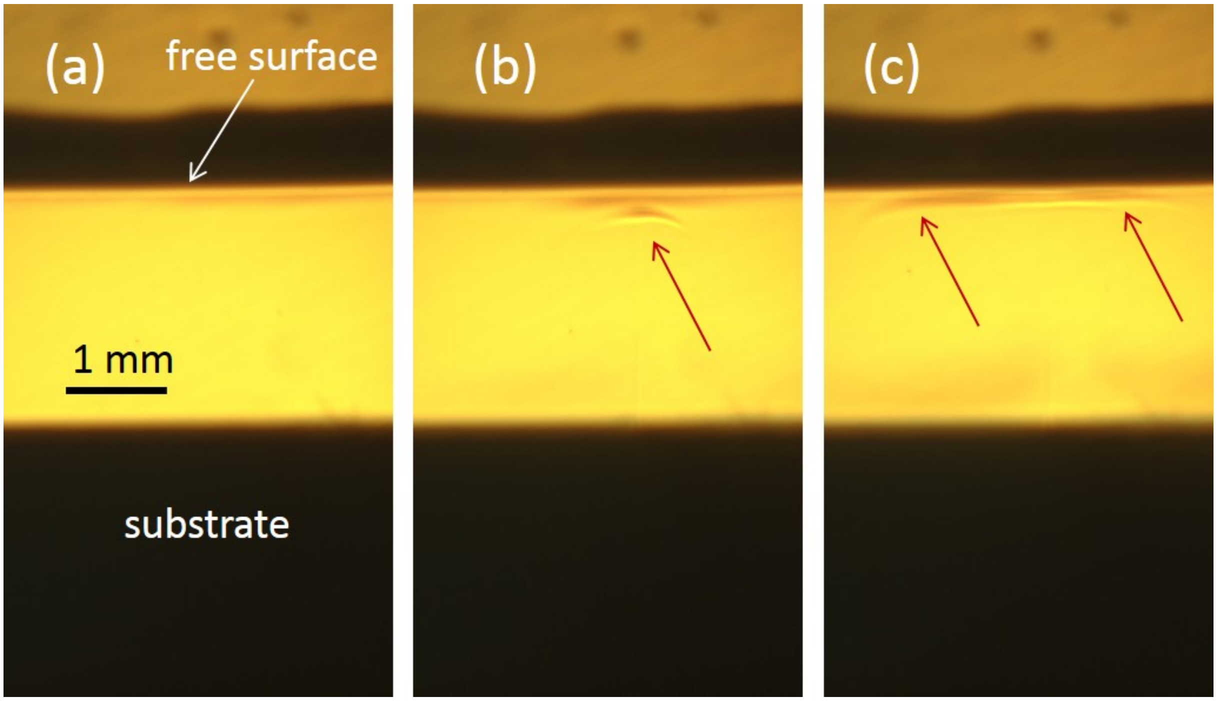


**Figure S1**. Schlieren contrast of nanobubbles collected near free liquid surface (indicated by the red arrows). The bubbles are produced by the pulses at frequency $f$ = 200 kHz with the voltage amplitude modulated by the triangle waveform. One cycle is 5 s long; the maximum amplitude is $U$ = 11 V. (a) Before the electrochemical process is started. (b) After one cycle. (c) After two cycles.

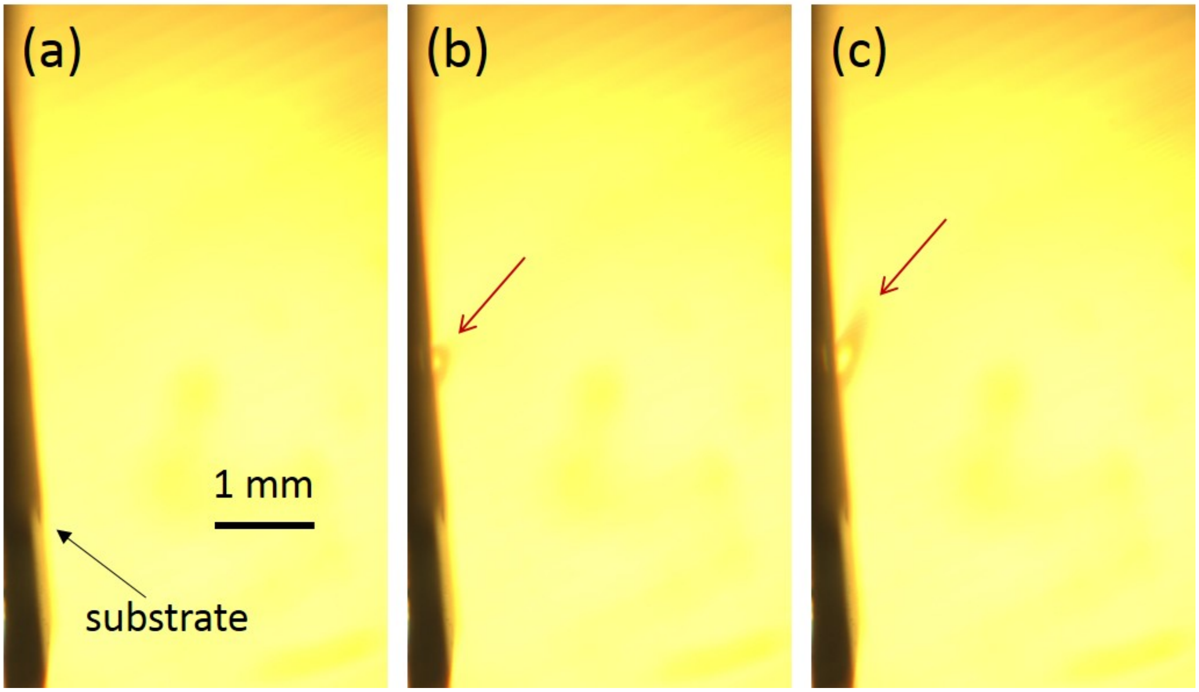


**Figure S2.** Buoyancy effect when the substrate is fixed vertically (along the direction of gravity). The nanobubbles are produced at the same conditions as in Figure S1. Position of the cloud of nanobubbles is indicated by the red arrows. The images (a), (b), and (c) correspond to the moment of time $t$ = 0 s, $t$ = 1.25 s, and $t$ = 2.5 s, respectively.
